# Supplementary material for: Two charges on plane in a magnetic field: II. Moving neutral quantum system across a magnetic field
Source: arXiv:1404.3333 source file (2014-07-10)
Supplement: Supplementary file 1 [file Supplementary-File.pdf]

| $P$ | $A_0$ | | | |
|---|---|---|---|---|
| | $B = 0.1$ | $B = 10$ | $B = 100$ | $B = 1000$ |
| 1 | 0.48 | 8.04 | 12.09 | 203.00 |
| 25 | −0.05 | 3.36 | 2.10 | 172.15 |
| 50 | −0.50 | 0.21 | −15.37 | 120.62 |
| 75 | −1.05 | −2.01 | −47.10 | 72.75 |
| 100 | – | −5.16 | −87.06 | 28.66 |
| 125 | – | −8.59 | −122.12 | −25.26 |
| 150 | – | −9.69 | −167.36 | −82.73 |
| 175 | – | −10.41 | −214.00 | −139.71 |
| 200 | – | – | −269.18 | −184.02 |

Table VII: Ground state. Parameter $A_0$ in (38). For $B = 1$, parameter $A_0 = 0.81$ for all $P$ considered. Magnetic field in effective atomic units, $B_0 = 9.3917 \times 10^9\, G$.

| $P$ | $A_2$ | | | |
|---|---|---|---|---|
| | $B=1$ | $B=10$ | $B=100$ | $B=1000$ |
| 1 | 0 | $-0.001$ | $-0.001$ | $-0.019$ |
| 25 | $-0.02$ | $-0.047$ | $-0.141$ | $-0.194$ |
| 50 | $-0.04$ | $-0.094$ | $-0.276$ | $-1.086$ |
| 75 | $-0.07$ | $-0.141$ | $-0.398$ | $-1.725$ |
| 100 | $-0.09$ | $-0.187$ | $-0.504$ | $-2.363$ |
| 125 | – | $-0.235$ | $-0.613$ | $-3.233$ |
| 150 | – | $-0.282$ | $-0.705$ | $-3.881$ |
| 175 | – | $-0.330$ | $-0.798$ | $-4.373$ |
| 200 | – | – | $-0.891$ | $-4.959$ |

Table VIII: Ground state. Parameter $A_2$ in (38). For $B = 0.1$, parameter $A_2 = 0$ for all $P$ considered. Magnetic field in effective atomic units, $B_0 = 9.3917 \times 10^9\, G$.

| $P$ | $A_3$ | | |
|---|---|---|---|
| | $B = 0.1$ | $B = 100$ | $B = 1000$ |
| 1 | 0.12 | 6.40 | 18.476 |
| 25 | 0.1 | 6.38 | 21.031 |
| 50 | 0.1 | 6.30 | 23.004 |
| 75 | 0.1 | 6.14 | 23.587 |
| 100 | – | 5.97 | 24.107 |
| 125 | – | 5.85 | 24.906 |
| 150 | – | 5.71 | 24.930 |
| 175 | – | 5.61 | 24.510 |
| 200 | – | 5.52 | 24.282 |

Table IX: Ground state. Parameter $A_3$ in (38). For $B = 1$, 10, parameter $A_3 = 0.75$, 2.02 respectively, for all $P$ considered. Magnetic field in effective atomic units, $B_0 = 9.3917 \times 10^9\, G$.

| $P$ | $A_4$ | | | |
|---|---|---|---|---|
| | $B=1$ | $B=10$ | $B=100$ | $B=1000$ |
| 1 | 0 | 0 | 0 | $-0.0003$ |
| 25 | $-0.01$ | $-0.004$ | $-0.003$ | $-0.0099$ |
| 50 | $-0.02$ | $-0.007$ | $-0.0058$ | $-0.0156$ |
| 75 | $-0.03$ | $-0.011$ | $-0.0073$ | $-0.0202$ |
| 100 | $-0.04$ | $-0.014$ | $-0.0080$ | $-0.0253$ |
| 125 | – | $-0.017$ | $-0.0087$ | $-0.0308$ |
| 150 | – | $-0.02$ | $-0.0089$ | $-0.0334$ |
| 175 | – | $-0.0235$ | $-0.0090$ | $-0.0347$ |
| 200 | – | – | $-0.0090$ | $-0.0369$ |

Table X: Ground state. Parameter $A_4$ in (38). For $B = 0.1$, parameter $A_4 = 0$ for all $P$ considered. Magnetic field in effective atomic units, $B_0 = 9.3917 \times 10^9\, G$.

| $P$ | $A_5$ | | |
|---|---|---|---|
| | $B=10$ | $B=100$ | $B=1000$ |
| 1 | 0.755 | 1.254 | 4.039 |
| 25 | 0.720 | 1.221 | 3.850 |
| 50 | 0.706 | 1.153 | 3.445 |
| 75 | 0.693 | 1.053 | 3.198 |
| 100 | 0.677 | 0.955 | 3.100 |
| 125 | 0.666 | 0.891 | 3.058 |
| 150 | 0.663 | 0.820 | 2.904 |
| 175 | 0.661 | 0.764 | 2.736 |
| 200 | – | 0.7144 | 2.637 |

Table XI: Ground state. Parameter $A_5$ in (38). For $B = 0.1$, 1, parameter $A_5 = 0.1$, 0.58 respectively, for all $P$ considered. Magnetic field in effective atomic units, $B_0 = 9.3917 \times 10^9\,G$.

| $P$ | $\alpha$ | | |
|---|---|---|---|
| | $B=10$ | $B=100$ | $B=1000$ |
| 1 | 32.42 | 126.13 | 321.74 |
| 25 | 30.20 | 122.58 | 302.54 |
| 50 | 28.14 | 119.72 | 283.12 |
| 75 | 26.94 | 115.05 | 261.19 |
| 100 | 25.20 | 110.43 | 229.17 |
| 125 | 22.74 | 104.93 | 180.53 |
| 150 | 21.93 | 100.99 | 145.58 |
| 175 | 21.44 | 95.12 | 117.62 |
| 200 | – | 85.00 | 92.93 |

Table XII: Ground state. Parameter $\alpha$ in (38). For $B = 0.1$, 1, parameter $\alpha = 1$, 2.45 respectively, for all $P$ considered. Magnetic field in effective atomic units, $B_0 = 9.3917 \times 10^9\, G$.

| $D$ | $B=0.1$ | $B=1$ | $B=10$ |
|---|---|---|---|
| $D_0$ | 1.39 | 0.93 | −0.998 |
| $D_1$ | 0.89 | 1.76 | 9.014 |
| $D_2$ | 0.89 | 1.76 | 9.014 |
| $D_3$ | 0.2384 | 0.9066 | 3.1228 |
| $D_4$ | 1.13 | 1.65 | 1.952 |
| $D_5$ | 1.13 | 1.64 | 1.952 |
| $D_6$ | 0.5692 | 0.8228 | 0.97624 |

Table XIII: Ground state. Parameters $D$'s in (38) for Pseudomomentum $P_c < P < 200$. Magnetic field in effective atomic units, $B_0 = 9.3917 \times 10^9\, G$.
